# Supplementary material for: Performance Analysis of Traditional and Data-Parallel Primitive Implementations of Visualization and Analysis Kernels
Source: arXiv:2010.02361 source file (2020-10-05)
Supplement: Supplementary file 1 [file appendix-perfCounters.tex]

%\onecolumn
\section{Hardware Performance Counters}
\label{sec:appendix-perfCounters}

%This is some text. 
\begin{table}[h!]
   \caption{Hardware performance counters and other measures we use in our experiments. }
    %\fix{this table needs to be updated, and possibly condensed. }}
    \label{table:perfCounters}
\footnotesize
    \centering
    \begin{tabular}{p{1.0in}cp{3.5in}}
    Performance counter, measure & Source & Description \\
    \hline
 \texttt{INSTR\_RETIRED\_ANY} & LIKWID & The Instructions Retired Any event that shows how many instructions were completely executed, and does not include speculative instruction loads~\cite{instRetiredEventWeb:2020}. \\
    \\
\texttt{FLOPS, FLOPS\_DP, FLOPS\_SP} & LIKWID &  The KNL platform the Xeon Phi (Knights Landing) provides no possibility to differentiate between double and single precision FLOP/s~\cite{LIKWID-website:2020}. Therefore, on KNL, we use the sum of 
    \texttt{UOPS\_RETIRED\_SCALAR\_SIMD} and \texttt{UOPS\_RETIRED\_PACKED\_SIMD} as a measure of the number of floating point operations executed. These counters may include integer arithmetic instructions as well. 
    On the Ivy Bridge platform, a sum of the performance counters
    \texttt{FP\_COMP\_OPS\_EXE\_SSE\_FP\_PACKED\_DOUBLE},
    \texttt{FP\_COMP\_OPS\_EXE\_SSE\_FP\_SCALAR\_DOUBLE},
    \texttt{SIMD\_FP\_256\_PACKED\_DOUBLE} capture both scalar and vector FP operations.
    On the Ivy Bridge, there is the known potential for inaccuracies with these measures, whereby the counters may include both instructions issued and retired. For the purposes of the test results we show here, we assume some ``error bars`` on the results, but consider the results informative within the broader context that considers counts of both FLOPs and other instructions executed. \\
    \\
Cycles Per Instruction (CPI) & LIKWID & Computed as the quotient of CPU\_CLK\_UNHALTED\_CORE / INSTR\_RETIRED\_ANY to give an estimate of the number of clock cycles per instruction.  \\
\\
Vectorization ratio  & LIKWID &  This value is the ratio of ``packed'' FLOPS to the sum  of all FLOPS. On the Ivy Bridge, this value is reported by LIKWID using the counters
    \texttt{FP\_COMP\_OPS\_EXE\_SSE\_FP\_PACKED\_DOUBLE},
    \texttt{FP\_COMP\_OPS\_EXE\_SSE\_FP\_SCALAR\_DOUBLE},
    \texttt{SIMD\_FP\_256\_PACKED\_DOUBLE}. On KNL, we compute vectorization ratio as \texttt{UOPS\_RETIRED\_PACKED\_SIMD} / (\texttt{UOPS\_RETIRED\_PACKED\_SIMD} + \texttt{UOPS\_RETIRED\_SCALAR\_SIMD)}. Note that on the KNL platform, the \texttt{UOPS\_RETIRED\_*} counters may include integer arithmetic as well as floating point instructions~\cite{LIKWID-website:2020}. \\
    \\
%\texttt{L2CACHE} & LIKWID &  This group measures the locality of data accesses with regard to the L2 cache. It reports the L2 request rate, L2 miss rate, and L2 miss ratio~\cite{LIKWID-website:2020}. \\
%\\
\texttt{L3CACHE} & LIKWID &  This group measures the locality of your data accesses with regard to the L3 cache. It reports the L3 request rate, L3 miss rate, and L3 miss ratio~\cite{LIKWID-website:2020}. Since the KNL has no L3 cache, this counter is not present on that platform. \\
%MEM_LOAD_UOPS_RETIRED_L3_ALL MEM_LOAD_UOPS_RETIRED_L3_MISS. 
 \\
%Memory footprint & \texttt{/usr/bin/time -v} & Reports various useful statistcs, including maximum resident set size (max RSS). \\
%    \\
Runtime & LIKWID and custom & We make use of LIKWID's ``marker API'' to restrict measurement to specific regions of code, namely the portion that performs computation of interest (stencil, isocontour, particle advection). We also make use of custom instrumentation in the codes to measure elapsed time using high-resolution timers, again to restrict measurement to a specific region of code. \\
\\
    \end{tabular}
\end{table}
